# Supplementary material for: Towards Real Smart Apps: Investigating Human-AI Interactions in Smartphone On-Device AI Apps
Source: arXiv:2307.00756 source file (2023-07-03)
Supplement: Supplementary file 1 [file 10-Appendix.tex]

% \section{Appendix}
\begin{appendices}
\label{Appendix}

\section{Title suggestions:}
\label{sec:titles}

\jason{Some Keywords: ``Practical”; ``Empirical ”; ``Real AI smart apps”; ``Human-AI interaction feedback”; ``Interaction patterns”. I think we can use the word of ``Give-And-Take"}
\begin{itemize}
	\item \jason{  Understanding Human-AI interaction feedback in real smart apps }
	\item \jason{  An empirical investigation into Human-AI interaction feedback in real smart apps}
	\item \jason{  Human-AI interaction patterns and where to find them: a study on AI smart apps and end-user feedback}
	\item \jason{  Practical Interaction patterns between AI smart apps and end-user feedback: Towards an empirical approach.}
	\item \jason{  Towards a closer dialogue between AI smart apps and end-user: A taxonomy of interaction patterns}
	\item \jason{  Better behaviors with end-users: A taxonomy of Human-AI feedback in real smart apps}
	\item \jason{  Better Give-and-take: A taxonomy of Human-AI feedback in real smart apps}
	\item \jason{  Exploring a better Give-and-take: A taxonomy of Human-AI feedback in real smart apps}
	\item \jason{  Need a better Give-and-take? A taxonomy of Human-AI feedback in real smart apps	}
	\item \jason{  Crossing human-AI boundary: A taxonomy of Human-AI feedback in real smart apps}
	\item \jason{  Real AI smart apps pay it forward? A taxonomy of End-user-AI feedback}
	\item Real AI smart apps pay it forward? A taxonomy of End-user-AI feedback \jason{(Here Pay-it-forward means do something beneficial to end-user)}
	\item A tale of reciprocity: Investigate Human-AI Interactions in Mobile Apps \jason{(Here reciprocity means do AI models [i.e., Better model performance] exchanges things with user [i.e., Use Experience] for mutual benefits. )}
	\item \jason{  A first look at Human-AI interaction on real smart apps}
	\item \jason{  Pay-It-Forward or Give-And-Take? A first look at Human-AI interaction on real smart apps}
	\item \jieshan{Guide me or not? An empirical study on Human-AI interaction for AI-support apps}
\end{itemize}

\end{appendices}
